# Supplementary material for: Exact Partitioning of High-order Planted Models with a Tensor Nuclear Norm Constraint
Source: arXiv:2006.11666 source file (2020-06-20)
Supplement: Supplementary file 1 [file 9_appendix.tex]

%\onecolumn
\newpage
\appendix
